# Supplementary material for: Smart Build Targets Batching Service at Google
Source: arXiv:2102.09098 source file (2021-02-18)
Supplement: Supplementary file 1 [file appendix.tex]

\clearpage
